# Supplementary material for: $E_8$ Spectra of Quasi-one-dimensional Antiferromagnet BaCo$_2$V$_2$O$_8$ under Transverse Field
Source: arXiv:2005.13302 source file (2021-08-10)
Supplement: Supplementary file 1 [file BCVO_SM.pdf]

[Supplemental Material]

# $E_8$ Spectra of Quasi-one-dimensional Antiferromagnet $BaCo_2V_2O_8$ under Transverse Field

Haiyuan Zou[1], Yi Cui[2], Xiao Wang[1], Z. Zhang[1], J. Yang[1], G. Xu[3], A. Okutani[4], M. Hagiwara[4], M. Matsuda[5], G. Wang[6], Giuseppe Mussardo[7], K. Hódsági[8], M. Kormos[9], Zhangzhen He[10], S. Kimura[11], Rong Yu[2], Weiqiang Yu[2], Jie Ma[12], and Jianda Wu[1,13]

*[1]Tsung-Dao Lee Institute, Shanghai Jiao Tong University, Shanghai, 200240, China*
*[2]Department of Physics and Beijing Key Laboratory of Opto-electronic Functional Materials & Micro-nano Devices, Renmin University of China, Beijing, 100872, China*
*[3]NIST Center for Neutron Research, National Institute of Standards and Technology, Gaithersburg, MD, 20899-6102, USA*
*[4]Center for Advanced High Magnetic Field Science, Graduate School of Science, Osaka University, Toyonaka, Osaka 560-0043, Japan*
*[5]Neutron Scattering Division, Oak Ridge National Laboratory, Oak Ridge, Tennessee 37831, USA*
*[6]Beijing National Laboratory for Condensed Matter Physics, Institute of Physics, Chinese Academy of Sciences, Beijing 100190, China*
*[7]SISSA and INFN, Sezione di Trieste, Via Bonomea 265, I-34136 Trieste, Italy*
*[8]BME-MTA Statistical Field Theory Research Group, Institute of Physics, Budapest University of Technology and Economics, 1111 Budapest, Budafoki út 8, Hungary*
*[9]MTA-BME Quantum Dynamics and Correlations Research Group, Department of Theoretical Physics, Budapest University of Technology and Economics, 1111 Budapest, Budafoki út 8, Hungary*
*[10]State Key Laboratory of Structural Chemistry, Fujian Institute of Research on the Structure of Matter, Chinese Academy of Sciences, Fuzhou, Fujian 350002, China*
*[11]Institute for Materials Research, Tohoku University, Sendai, Miyagi 980-8577, Japan*
*[12]Key Laboratory of Artificial Structures and Quantum Control (Ministry of Education), Shenyang National Laboratory for Materials Science, School of Physics and Astronomy, Shanghai Jiao Tong University, Shanghai, 200240, China*
*[13]School of Physics & Astronomy, Shanghai Jiao Tong University, Shanghai, 200240, China*

## S1. Methods

Single crystals of $BaCo_2V_2O_8$ (BCVO) were grown by the flux method (NMR) and the floating zone method (INS). The NMR crystal has a dimension of 2mm*1.5mm*0.5mm along, whose orientation is determined by the Laure spectroscopy. The crystal used for the INS experiments is rod-shaped with 6 mm in diameter and 40 mm in length.

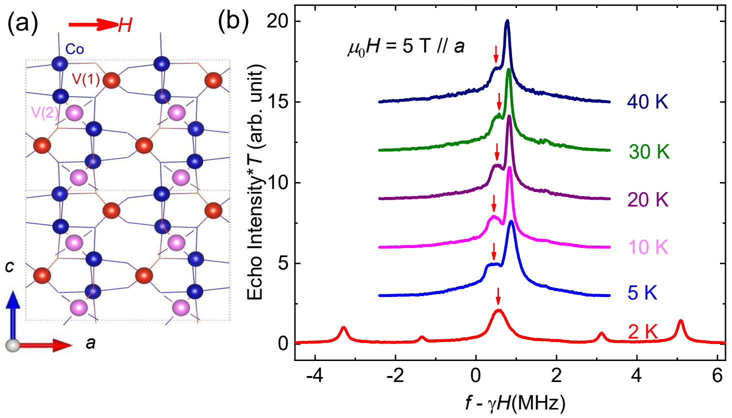


**Fig. S1:** (a) Illustration of two inequivalent vanadium sites V(1) and V(2), with field along the crystalline *a* axis. (b) The $^{51}$V NMR spectra at typical temperatures, measured under an in-plane field of 5 T applied along the *a*-axis. The center frequency $^{51}\gamma H$ = 55.9 MHz. The spectra are shifted vertically for clarity. The integrated spectral intensity is multiplied by temperature, which conserves as a constant due to Zeeman distribution. The down arrows mark the left peak, which is tentatively assigned to be site V(2) (see text).

The $^{51}$V ($I = 7/2$, $^{51}\gamma = 11.198$ MHz/T) NMR spectra are measured under a transverse magnetic field applied along the crystalline $a$ axis, by integrating the spin-echo signal with frequency sweeps. Note that at zero field, all Vanadium sites are equivalent in the paramagnetic phase. Under a finite field, however, the vanadium sites are inequivalent in the paramagnetic phase, as labeled by V(1) and V(2) in Fig. S1(a), respectively. Fig. S1(b) depicts the $^{51}$V NMR spectra with temperature at a typical field of 5 T, which is below the 3D quantum critical point. At high temperatures, each spectrum consists of two peaks, consistent with the two inequivalent $^{51}$V in the paramagnetic state, with field along the [010] direction. Note that the quadrupole contribution is too small to cause any resolvable line splitting in the spectrum at the measured temperatures. Further line splitting at 2 K is an evidence for the magnetic ordering.

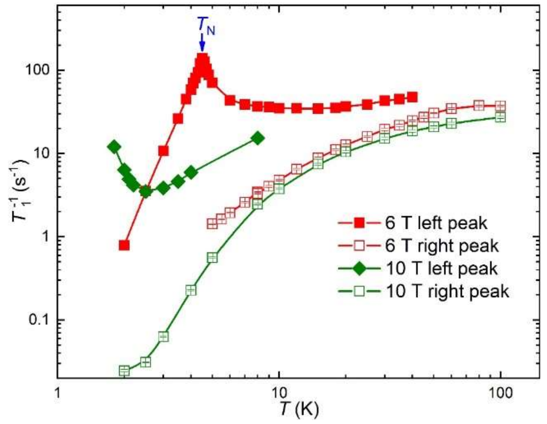


**Fig. S2**: The $1/T_1$ as functions of temperatures, measured on two NMR peaks seen in Fig. S1(b), with fields applied along the crystalline $a$ axis. $T_N$ labels the magnetic transition temperature under field.

The spin-lattice relaxation time $T_1$ is measured by the saturation-recovery method with a single $\pi/2$ pulse as the saturation pulse. The recovery curve is fit by the stretched exponential function $I(t)/I(0) = 1 - a[0.01191e^{-\left(\frac{t}{T_1}\right)^\beta} + 0.06818e^{-\left(\frac{6t}{T_1}\right)^\beta} + 0.20604e^{-\left(\frac{15t}{T_1}\right)^\beta} + 0.71387e^{-\left(\frac{28t}{T_1}\right)^\beta}]$, for spin-7/2 nuclei [1,2]. where $\beta$ is the stretching factor which is about 1 above $T_N$ and less than 1 below $T_N$. $\beta$ is found to be 1 with temperatures from 6 K to 12 K at the measured fields, which is the region to determine the 1D quantum critical behavior.

The spin-lattice relaxation rate $1/T_1$ is measured at the two NMR peaks in Fig.S1 (b), and the temperature dependence of the data is plotted in Fig. S2. $1/T_1$ measured at the left NMR peak exhibits a dramatic increase and a peaked behavior when cooled toward the Néel temperature $T_N$, signaling enhanced critical spin fluctuations. However, the low-temperature $1/T_1$ measured at the right NMR peak is over one-order of magnitude lower and barely sense the magnetic transition. Therefore, in the main text, we report the $T_1$ of the left peak of the spectrum, which is more appropriate for the study of quantum criticality.

We assign the left peak of the spectra, labeled by red arrows in Fig. S1(b), to the vanadium site V(2) shown in Fig. S1(a), and the right peak to the V(1) site. The reason is as follows. As reported earlier [3,4], the hyperfine field on a vanadium nucleus in $BaCo_2V_2O_8$ is found to be caused by a combination of a regular hyperfine contribution and an anisotropic dipolar contribution between the neighboring $Co^{2+}$ moments and the $^{51}$V nuclear spin. With the external field applied along the crystalline $a$ axis in the paramagnetic state, the regular hyperfine coupling is the same for all vanadium

sites, whereas the dipolar one is different for V(1) and V(2) sites [4]; that is, the total hyperfine field $H_{in}^{a} = (A_1 + A_2)m_a$, where $A_1$ is a positive constant, $A_2$ is the dipolar term which varies with sites, and $m_a$ is the paramagnetic moment of $Co^{2+}$ . We then calculated the dipolar coupling according to the atomic position and the field orientation, and found that $A_2 = 1.98a$ and $-2.18a$, for the V(1) site and V(2) site, respectively, where $a$ is a positive constant. Taking into account both the positive regular hyperfine coupling and the dipolar coupling, the value of $H_{in}$ is bigger for the V(1) than that for the V(2) site, as illustrated in Fig. S3(a). Then the low-frequency peak in Fig. S1(b) is reasonably attributed to V(2), and the high-frequency one is attributed to V(1).

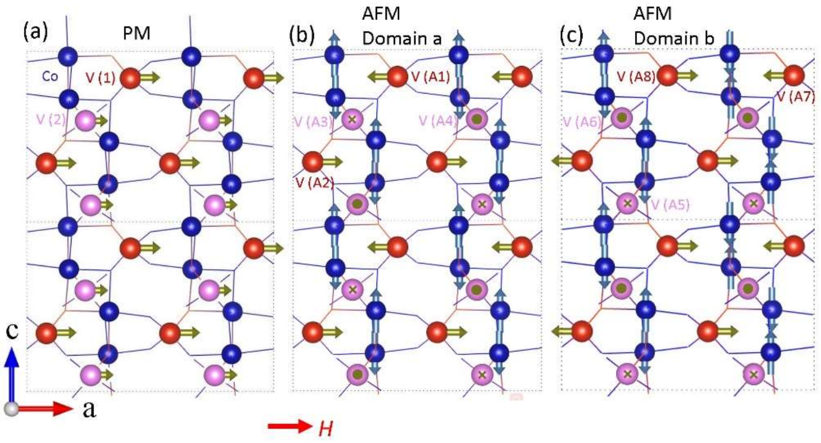


**Fig. S3:** Illustration of directions and amplitudes of hyperfine fields on vanadium nuclear spins, as shown by the Golden arrows, with the external magnetic field applied along the crystalline *a* axis. (a) In the high-temperature paramagnetic (PM) phase; (b) In the low-temperature antiferromagnetic phase with domain a; (b) In the low-temperature antiferromagnetic phase with domain b.

This above assignment can also explain the difference of the $1/T_1$ measured at the two peaks in Fig. S2. Before we discuss the antiferromagnetic (AFM) fluctuations just above $T_N$, we first consider the AFM phase of $BaCo_2V_2O_8$ below $T_N$ with the known magnetic structure. Following Ref. [3] and Ref. [4], the resulting internal hyperfine fields on each V nucleus, caused by the AFM ordering, are presented in Fig. S3 (b)-(c) with two types of magnetic domains of $BaCo_2V_2O_8$ [3]. The isotropic hyperfine field is found to be canceled out due to local geometric symmetry, whereas the dipolar hyperfine field varies among the sites. The hyperfine field vector is calculated to be $\vec{H}_{in} = (H_{in}^{a}, H_{in}^{b}, H_{in}^{c}) = (\pm 0.633, 0, 0)m$ or $\vec{H}_{in} = (\pm 0.779, 0, 0)m$ for site V(1) [labeled as V(A1), V(A2), V(A7) and V(A8)], and $\vec{H}_{in} = (0, \pm 0.633, 0)m$ or $\vec{H}_{in} = (0, \pm 0.779, 0)m$ for site V(2) [labeled as V(A3), V(A4), V(A5) and V(A6)], in either domain a or domain b [3], where $m$ is the amplitude of the ordered moment, and $a$, $b$, $c$ are orthogonal crystalline directions. Note that with the external field applied along the $a$ axis, in each domain, the local hyperfine field on the V(1) nuclear spin is parallel to the external field, while the hyperfine field on the V(2) nuclear spin is perpendicular to the external field. Since $1/T_1$ probes the hyperfine field fluctuations that are transverse to the external field, the $1/T_1$ on V(2) should measure the AFM fluctuations and $1/T_1$ on V(1) should be negligible as both $H_{in}^{b}$ and $H_{in}^{c}$ are zero.

In the paramagnetic phase, the domains are strongly fluctuating, which could cause additional contribution to $1/T_1$. But when approaching to $T_N$, $1/T_1$ should still be dominated by the AFM fluctuations, as just discussed above. Therefore, the critical behavior of $1/T_1$ at the left NMR peak again supports that the left peak is associated with the V(2) site. We

note that similar effect of the $1/T_1$ caused by dipolar hyperfine field has been addressed in explaining the stripe-type AFM fluctuations of the iron-based superconductors [5,6,7].

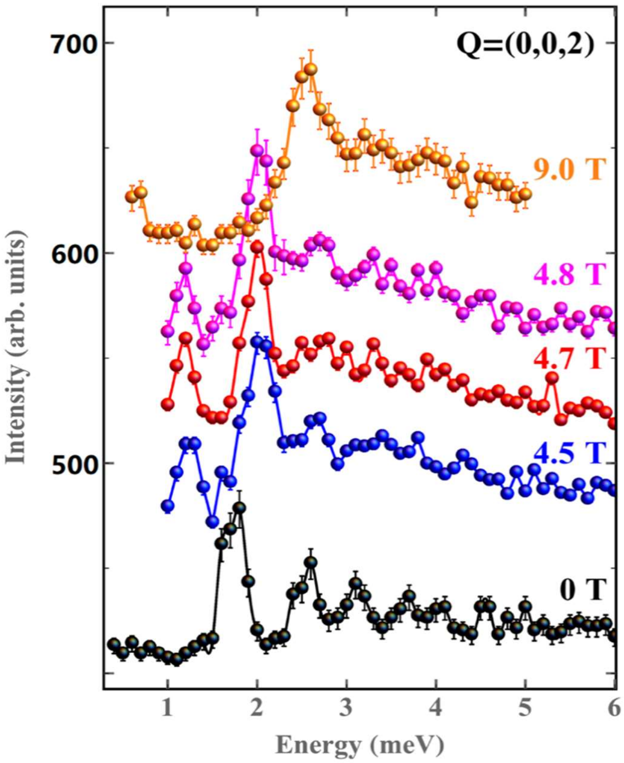


**Fig. S4:** Spin dynamical structure factor data measured by inelastic neutron scattering experiments with Q = (0,0,2) in BCVO at 0.4 K, under different transverse field along the [010] direction. Because of explicitly large data counting for energy larger than 3meV from 4.5T to 4.8T, the error bars are within the size of illustrated data points.

The inelastic neutron scattering measurements were taken at the Spin Polarized Inelastic Neutron Spectrometer (SPINS) at the NCNR and the cold neutron triple-axis spectrometer (CG-4C) at the High Flux Isotope Reactor (HFIR) at Oak Ridge National Laboratory (ORNL). A mass of ~2g single-crystal is aligned in (h0l) plane with the external field along the *b*-axis. For SPINS, the final energy was fixed at 5meV, with horizontal collimation of guide-open-sample-80'-open. The 10 T vertical magnet with orange cryostat (down to $T = 1.5$ K) and 7 T vertical magnet with $He^3$ refrigerator (down to $T = 0.4$ K) were applied, respectively. We obtained the spin dynamical structure factor for BCVO at different transverse fields (Fig. S4). The energy gap continuously decreases when field increases. $E_8$ physics appears at around $\mu_0 H = 4.7$T. For CG-4C, a final energy of 5 meV was used with a horizontal collimator sequence of guide-40'-40'-120'. For both instruments, the contamination from higher-order beams was effectively eliminated using Be filters.

## S2. Numerical Calculations

Consisting of screw-like chains of $Co^{2+}$ along the crystallographic $c$-axis, BCVO shows an antiferromagnetic (AF) structure with the $c$-axis at zero magnetic field, suggests an Ising-like one dimensional structure. The AF chain in BCVO in the transverse field is described by the spin-1/2 XXZ model with Hamiltonian [8,9]:

$$\mathcal{H} = J\sum_{n,i}[S^z_{n,i}S^z_{n+1,i} + \epsilon(S^x_{n,i}S^x_{n+1,i} + S^y_{n,i}S^y_{n+1,i})] - \mu_B \sum_{n,i} \tilde{g}\, \mathbf{H}\cdot\mathbf{S}_{n,i} + J'\sum_{n,i\neq j} S^z_{n,i}S^z_{n,j}, \qquad \text{(S1)}$$

where the first term is the $XXZ$ Hamiltonian with intrachain interaction coupling $J = 5.8$ meV, the anisotropic factor $\epsilon = 0.46$ for BCVO, $\mathbf{S} = \boldsymbol{\sigma}/2$, and $\boldsymbol{\sigma}$ refer to the three Pauli matrices. The second term is produced by the external magnetic field $\mathbf{H}$, with $\mu_B$ being the Bohr magneton and $\tilde{g}$ being the Lande tensor determined by the crystal structure. The third term is the interchain interaction with the coupling $J' > 0$. In the Hamiltonian, $n$ is site index, and $i, j$ label different chains.

Applying a transverse field along the [010] direction induces a staggered transverse field along the [100] direction and a four-period staggered field along the [001] direction, the second term of the Hamiltonian at a chain is then written as

$$\mu_B \sum_n \tilde{g}\, \mathbf{H}\cdot\mathbf{S}_n = \mu_B g_{yy} H \sum_n [S^y_n + h_x(-1)^n S^x_n + h_z \cos(\pi \tfrac{2n-1}{4}) S^z_n] \;, \qquad \text{(S2)}$$

with the gyromagnetic ratio $g_{yy} = 2.75$, the applied transverse field $H$, and the ratio of the induced fields to $\mu_B g_{yy} H$ are set as $h_{x(z)} = 0.4(0.14)$. The staggered transverse field suppresses the magnetic ordering significantly.

At the external magnetic field $\mu_0 H < 10$ T, the ground state of the Hamiltonian is an AF ordered state. Consider very weak interchain coupling in BCVO, we take mean-field approximation for the interchain interaction. Then the third term of the Eq. (S1) gives rise to a staggered longitudinal perturbation term with an effective field $H'$ as

$$J'\sum_{n,i\neq j} S^z_{n,i}S^z_{n,j} \rightarrow -\mu_B H' \sum_n (-1)^n S^z_n \;. \qquad \text{(S3)}$$

With the chain mean-field approximation in Eq. (S3), we obtain a one-dimensional effective model to describe the system within the ordering dome as follows [Eq. (1) in main text],

$$\mathcal{H} = J\sum_n[S^z_nS^z_{n+1} + \epsilon(S^x_nS^x_{n+1} + S^y_nS^y_{n+1})] - \mu_B g_{yy} H \sum_n \left[S^y_n + h_x(-1)^n S^x_n + h_z \cos\left(\pi\frac{2n-1}{4}\right) S^z_n\right] - \mu_B H' \sum_n (-1)^n S^z_n \;, \qquad \text{(S4)}$$

where the effective field $H'$ can be determined self-consistently [9].

Following the effective Hamiltonian of Eq.S4, we then calculate zero-temperature space-time correlation $\langle S^\mu(\boldsymbol{r},t)S^\nu(\mathbf{0},0)\rangle$ using infinite time-evolving block decimation (iTEBD) [10]. The Fourier transform of the correlation function

$$D^{\mu\nu}(\omega,\boldsymbol{Q}) = \int dt \sum_r e^{i(\omega t - \boldsymbol{Q}\cdot\boldsymbol{r})} \langle S^\mu(\boldsymbol{r},t)S^\nu(\mathbf{0},0)\rangle \qquad \text{(S5)}$$

is related with the differential neutron scattering cross section (intensity) as

$$\frac{d^2\sigma}{d\Omega dE} \propto \frac{|q_f|}{|q_i|}\sum_{\mu,\nu=x,y,z}\left(\delta_{\mu\nu} - \frac{Q_\mu Q_\nu}{|\boldsymbol{Q}|^2}\right)|F(\boldsymbol{Q})|^2 D^{\mu\nu}(\omega,\boldsymbol{Q}), \qquad \text{(S6)}$$

where $F(\boldsymbol{Q})$ is the magnetic form factor and the scattering vector $\boldsymbol{Q}$ is defined as $\boldsymbol{Q} = q_i - q_f$ with $q_i, q_f$ as the initial and final wave vectors, respectively. In our numerical calculation, we set $|q_i| = |q_f|$ and assume a uniform form factor. For different scattering direction $\boldsymbol{Q}$, $D^{\mu\mu}(\omega, \boldsymbol{Q})$ $(\mu = x, y, z)$ contributes to the neutron cross section with different weight [11]. For example, the intensity contains 100%, 99.3% and 0.7% of $D^{yy}$, $D^{xx}$ and $D^{zz}$ components at the zone centre (ZC) position $\boldsymbol{Q}$=(0,0,2). We ignore the small cross term $D^{\mu\nu}(\omega, \boldsymbol{Q})$ $(\mu \neq \nu)$ [9].

Without taking into account the interchain coupling, a QCP of TFIC universality is theoretically calculated to arise around 5 T, according to the detailed infinite time-evolving block decimation (iTEBD) [10,11,12], which is consistent with the NMR data [Fig. 2 in the main text]. The interchain coupling shifts the true 3D quantum phase transition to be around 10 T in BCVO [see Fig. 1(b) in the main text] [9,11]. This implies that inside the 3D AF phase, the effective staggered field $H'$ perturbs the 1D QCP, provides a necessary factor for the desired $E_8$ excitations.

Starting from the configuration near the TFIC phase transition of the effective 1D model [Eq. (S1)] without the mean-field $H'$ term and then adding an effective field $\mu_B H' = 0.018J$ [9], we obtain the ground state in the $E_8$ region. In the iTEBD calculations, the bond dimension is $\chi = 45$, and the discretized time interval for time evolution is $dt = 0.02J^{-1}$. Calculation of the correlation function is numerically expensive in general. A usual practical approach is to extrapolate the correlation function to longer times with linear predictions [12], which produces the spectrum with few frequencies [13]. However, it is too artificial to extrapolate the correlation with larger numbers of frequencies, e.g. all the frequencies of many-body excitations of $E_8$ particles. Thus, we take large number of steps for time evolution, up to 10000 steps and Fourier transform the correlation functions without any extrapolation.

We also calculate the dynamical structure factor and the corresponding neutron scattering intensity for the system without the induced small component along the $c$-axis [the $h_z$ term in Eq. (S2)] and find that the effect of the $h_z$ term is negligible, which is consistent with the previous study on the universality of the quantum phase transition [14] and the dynamical structure factor [9].

Our intensity results excellently agree with the experimental data of all the single- and multi-quasiparticle excitation with energy up to $m_8$. Furthermore, the additional peaks observed in experiment from zone folding effect are also emerged in the numerical simulation [Fig. 3(c) in main text], i.e. an additional peak $F_1$ in between $m_3$ and $m_4$ is from $q = 0$ and $F_2$ (coincidence with $P_{13}$) is from $q = \pi/2$. These iTEBD results indeed validate the model Hamiltonian and support the $E_8$ physics hiding in BCVO.

## S3. Theoretical Analysis

The identified 1D QCP belongs to the transverse field Ising chain universality class [9], thus the emergent physics at the QCP is controlled by the conform field theory with central charge $c = 1/2$. Due to the antiferromagnetic nature of the Ising coupling along the chain in the material, for emerging quantum $E_8$ integrable model, a staggered longitudinal field is needed to couple to the relevant field. Fortunately, the 3D AF ordering now provides such an effective staggered longitudinal field. As such the physics around the masked 1D QCP can now be described by the central charge 1/2 CFT perturbed by the relevant field [15,16,17]:

$$\mathcal{H}_{E_8} = \mathcal{H}_{1/2} + h\int \sigma(x)dx, \qquad \text{(S7)}$$

where $\mathcal{H}_{1/2}$ is the Hamiltonian of the $c = 1/2$ CFT, and the second term is a perturbation from the field $\sigma(x)$ with coupling $h$ [16].

| $\|n\rangle$ | the total energy reduced by $m_1$ | $\|n\rangle$ | the total energy reduced by $m_1$ |
|---|---|---|---|
| $A_1$ | 1 | $A_2A_5$ | ≥4.5743 |
| $A_2$ | 1.6180 | $A_2A_6$ | ≥4.8364 |
| $A_3$ | 1.9890 | $A_3A_3$ | ≥3.9781 |
| $A_4$ | 2.4049 | $A_3A_4$ | ≥4.3939 |
| $A_5$ | 2.9563 | $A_3A_5$ | ≥4.9453 |
| $A_6$ | 3.2183 | $A_4A_4$ | ≥4.8097 |
| $A_7$ | 3.8912 | $A_1A_1A_1$ | ≥3 |
| $A_8$ | 4.7834 | $A_1A_1A_2$ | ≥3.6180 |
| $A_1A_1$ | ≥2 | $A_1A_1A_3$ | ≥3.9890 |
| $A_1A_2$ | ≥2.6180 | $A_1A_1A_4$ | ≥4.4049 |
| $A_1A_3$ | ≥2.9890 | $A_1A_1A_5$ | ≥4.9563 |
| $A_1A_4$ | ≥3.4049 | $A_1A_2A_2$ | ≥4.2361 |
| $A_1A_5$ | ≥3.9563 | $A_1A_2A_3$ | ≥4.6071 |
| $A_1A_6$ | ≥4.2183 | $A_1A_3A_3$ | ≥4.9781 |
| $A_1A_7$ | ≥4.8912 | $A_2A_2A_2$ | ≥4.8541 |
| $A_2A_2$ | ≥3.2361 | $A_1A_1A_1A_1$ | ≥4 |
| $A_2A_3$ | ≥3.6071 | $A_1A_1A_1A_2$ | ≥4.6180 |
| $A_2A_4$ | ≥4.0229 | $A_1A_1A_1A_3$ | ≥4.9890 |

**Table S1:** The first 36 lowest-energy ($< 5m_1$) states entering the spectra series obtained from Eq. (S8). The subscript in $A_i$ in the first column labels the corresponding $E_8$ particle with mass $m_i$. The second column lists the characteristic energy or the lower-bound of the excitation. Although total momentum is zero, but an internal momentum distribution is allowed for particles in the multi-particle state. Therefore, the total energy carried by multi-particles is larger than the sum of static masses.

The universality of the original model allows one to use the effective integrable field model to describe the excitation in BCVO. We calculate the spin dynamic structure factors, e.g. for the zero-momentum transfer case:

$$D^{\alpha\alpha}(\omega, q = 0) = \sum_{n=0}^{\infty} \int_{-\infty}^{+\infty} \frac{d\theta_1 \cdots d\theta_n}{N(2\pi)^{n-2}} \left|\langle 0|\sigma^\alpha|A_{a_1}(\theta_1) \cdots A_{a_n}(\theta_n)\rangle\right|^2 \delta(\omega - E\{a_i\})\delta(P\{a_i\}), (\alpha = x, z), \quad \text{(S8)}$$

where $N = \prod_{i=1}^{8} n_i!$, $a_i = m_1, \cdots, m_8$ $(i = 1, \cdots, n)$ labels a particle with corresponding mass in the $E_8$ model. In addition, $E\{a_i\} = \sum_{i=1}^{n} a_i \cosh\theta_i$, and $P\{a_i\} = \sum_{i=1}^{n} a_i \sinh\theta_i$. We determine $D^{\alpha\alpha}(\omega, q = 0)$ with a cut-off energy in our calculation fixed at $\omega_{cut} = 5m_1$ (here $\hbar$ and $c$ are set as one, $m_1$ is the mass of the lightest particle in the model), which is above the threshold of two-particle excitation. To achieve this realistic goal, we calculate all contributed channels [cf. Table S1] within which the sum of particles' masses is smaller than $\omega_{cut}$. Following Ref. [18], $D^{yy}(\omega, q = 0)$ can be immediately obtained from $D^{zz}$.

As an illustration, the results for $D^{xx}(\omega, q = 0)$ are summarized in Fig. 3(d)-(g) (main text) with contribution from each independent single- or multi-particle channel, where the analytical data are broadened in a Lorentzian fashion with full-width at half-maximum fixed at $0.08m_1$ corresponding to 0.1 meV energy resolution in experiment with $m_1$ = 1.2 meV. The DSF spectra from each multi-particle channel form a continuum, however, every continuum has its own special feature. It is especially significant for the two-particle scattering channel [Fig. 3(e) in main text] where each one exhibits a clear peak near the threshold (sum of static masses) followed by a long tail. It can be clearly observed that the total of them leave us clear and distinguishable peaks, bumping up and down in the spectrum continuum region. These unique features can be directly observed in inelastic neutron experiments with proper resolution (Fig. 3 in main text).

In the following, we discuss the significant suppression of the $m_1$ peak in both the neutron data and the numerical results shown in Fig. 3 of the main text. Note that the single-particle $E_8$ peaks of the calculated DSF in the effective model (Eq. 2 of the main text) exhibit strong decay with increasing energy. Though the model of Eq. 2 describes the universal behavior near the TFIC, microscopic details of real materials may strongly affect the shape of the DSF. Here we show that the

observed strong suppression of the $m_1$ peak is caused by the spin-flip interaction. This interaction generally exists in real materials, and is described by the $\epsilon$ term in Eq. 1 of the main text. Analytically, its effects can be considered by adding the following term to the $E_8$ Hamiltonian of Eq. 2,

$$\mathcal{H} = \mathcal{H}_{E_8} + \epsilon_s \int \left(\sigma^x(x)\right)^2 dx, \tag{S9}$$

where $\epsilon_s$ corresponds to the $\epsilon$ in Eq.1 in the scaling limit. We treat the $\epsilon_s$ term as a perturbation, and calculate the correction to the DSF. To the 1st order, the correction to the $k$'s single-particle peak is [19]

$$\Delta D_k^{xx}(\omega, q = 0) \sim -\epsilon_s \frac{\langle 0|\sigma^x|A_{a_k}(0)\rangle}{m_k} G_k \delta(\omega - m_k), \tag{S10}$$

where

$$G_k = \sum_{i=1}^{8} \sum_{j=1}^{8} \left\langle A_{a_k}(0) \middle| \sigma^x \middle| A_{a_j}(0) \right\rangle \frac{\langle 0|\sigma^x|A_{a_j}(0)\rangle \langle A_{a_j}(0)|\sigma^x|A_{a_i}(0)\rangle}{m_{a_i}^2}. \tag{S11}$$

$|A_{a_i}(0)\rangle$ corresponds to a single particle state with zero rapidity. The first-order perturbation correction of DSF Eq. (S10) directly implies that the single particle peaks will be suppressed by the first-order correction. But the suppression for different types of $E_8$ excitations is inversely proportional to the mass of the particles, and proportional to the combination of form factors ($\langle 0|\sigma^x|A_{a_k}(0)\rangle G_k$) which decays exponentially fast with increasing masses. Therefore, only the lowest ($m_1$) peak suffers significant suppression. With the above perturbative calculation, we see that the analytical result is consistent with both the numerical and experimental ones.

## References


1. D. E. MacLaughlin, J. D. Williamson, and J. Butterworth, Phys. Rev. B 4, 60 (1971).
2. S. Wada, R. Aoki, and O. Fujita, J. Phys. F **14**, 1515 (1984).
3. Y. Kawasaki, Y. Ideta, Y. Kishimoto, T. Ohno, K. Omura,T. Fujita, S. Kimura, and M. Hagiwara, J. Phys. Soc. Japan **3**, 014001 (2014).
4. Y. Cui, H. Zou, N. Xi, Z. He, Y. X. Yang, L. Shu, G. H. Zhang, Z. Hu, T. Chen, R. Yu, J. Wu, and W. Yu, Phys. Rev. Lett. **123**, 067203 (2019).
5. K. Kitagawa, N. Katayama, K. Ohgushi, M. Yoshida, and M. Takigawa, J. Phys. Soc. Jpn. **77**, 114709 (2008).
6. S. Kitagawa, Y. Nakai, T. Iye, K. Ishida, Y. Kamihara, M. Hirano, and H. Hosono, Phys. Rev. B **81**, 212502 (2011).
7. P. S. Wang, S. S. Sun, Y. Cui, W. H. Song, T. R. Li, R. Yu, H. Lei, and W. Yu, Phys. Rev. Lett. **117**, 237001 (2016).
8. S. Kimura *et al.*, J. Phys. Soc. Jpn. **82**, 033706 (2013).
9. Q. Faure *et al.*, Nature Physics **14**, 716 (2018).
10. G. Vidal, Phys. Rev. Lett. **98**, 070201 (2007).
11. M. Matsuda *et al.*, Phys. Rev. B **96**, 024439 (2017).
12. S. R. White and I. Affleck, Phys. Rev. B **77**, 134437 (2008).
13. J. A. Kjäll, F. Pollmann, and J. E. Moore, Phys. Rev. B **83**, 020407(R) (2011).
14. H. Zou, R. Yu, and J. Wu, J. Phys: Condens Matter **32**, 045602 (2020).
15. A. B. Zamolodchikov, Int. J. Mod. Phys. A **4**, 4235 (1989).
16. G. Delfino and G. Mussardo, Nucl. Phys. B **455**, 724 (1995).
17. G. Delfino and P. Simonetti, Phys. Lett. B **383**, 450 (1996).
18. J. Wu, M. Kormos, and Q. Si, Phys. Rev. Lett. **113**,247201 (2014).
19. K. Hódsági, M. Kormos, and G. Takács, J. High Energy Phys. 2019, 047 (2019).
